# Supplementary material for: PanoMixSwap Panorama Mixing via Structural Swapping for Indoor Scene Understanding
Source: arXiv:2309.09514 source file (2023-09-27)
Supplement: Supplementary file 1 [file 06_supplementary.tex]

\begin{figure*}
\includegraphics[scale=.275]{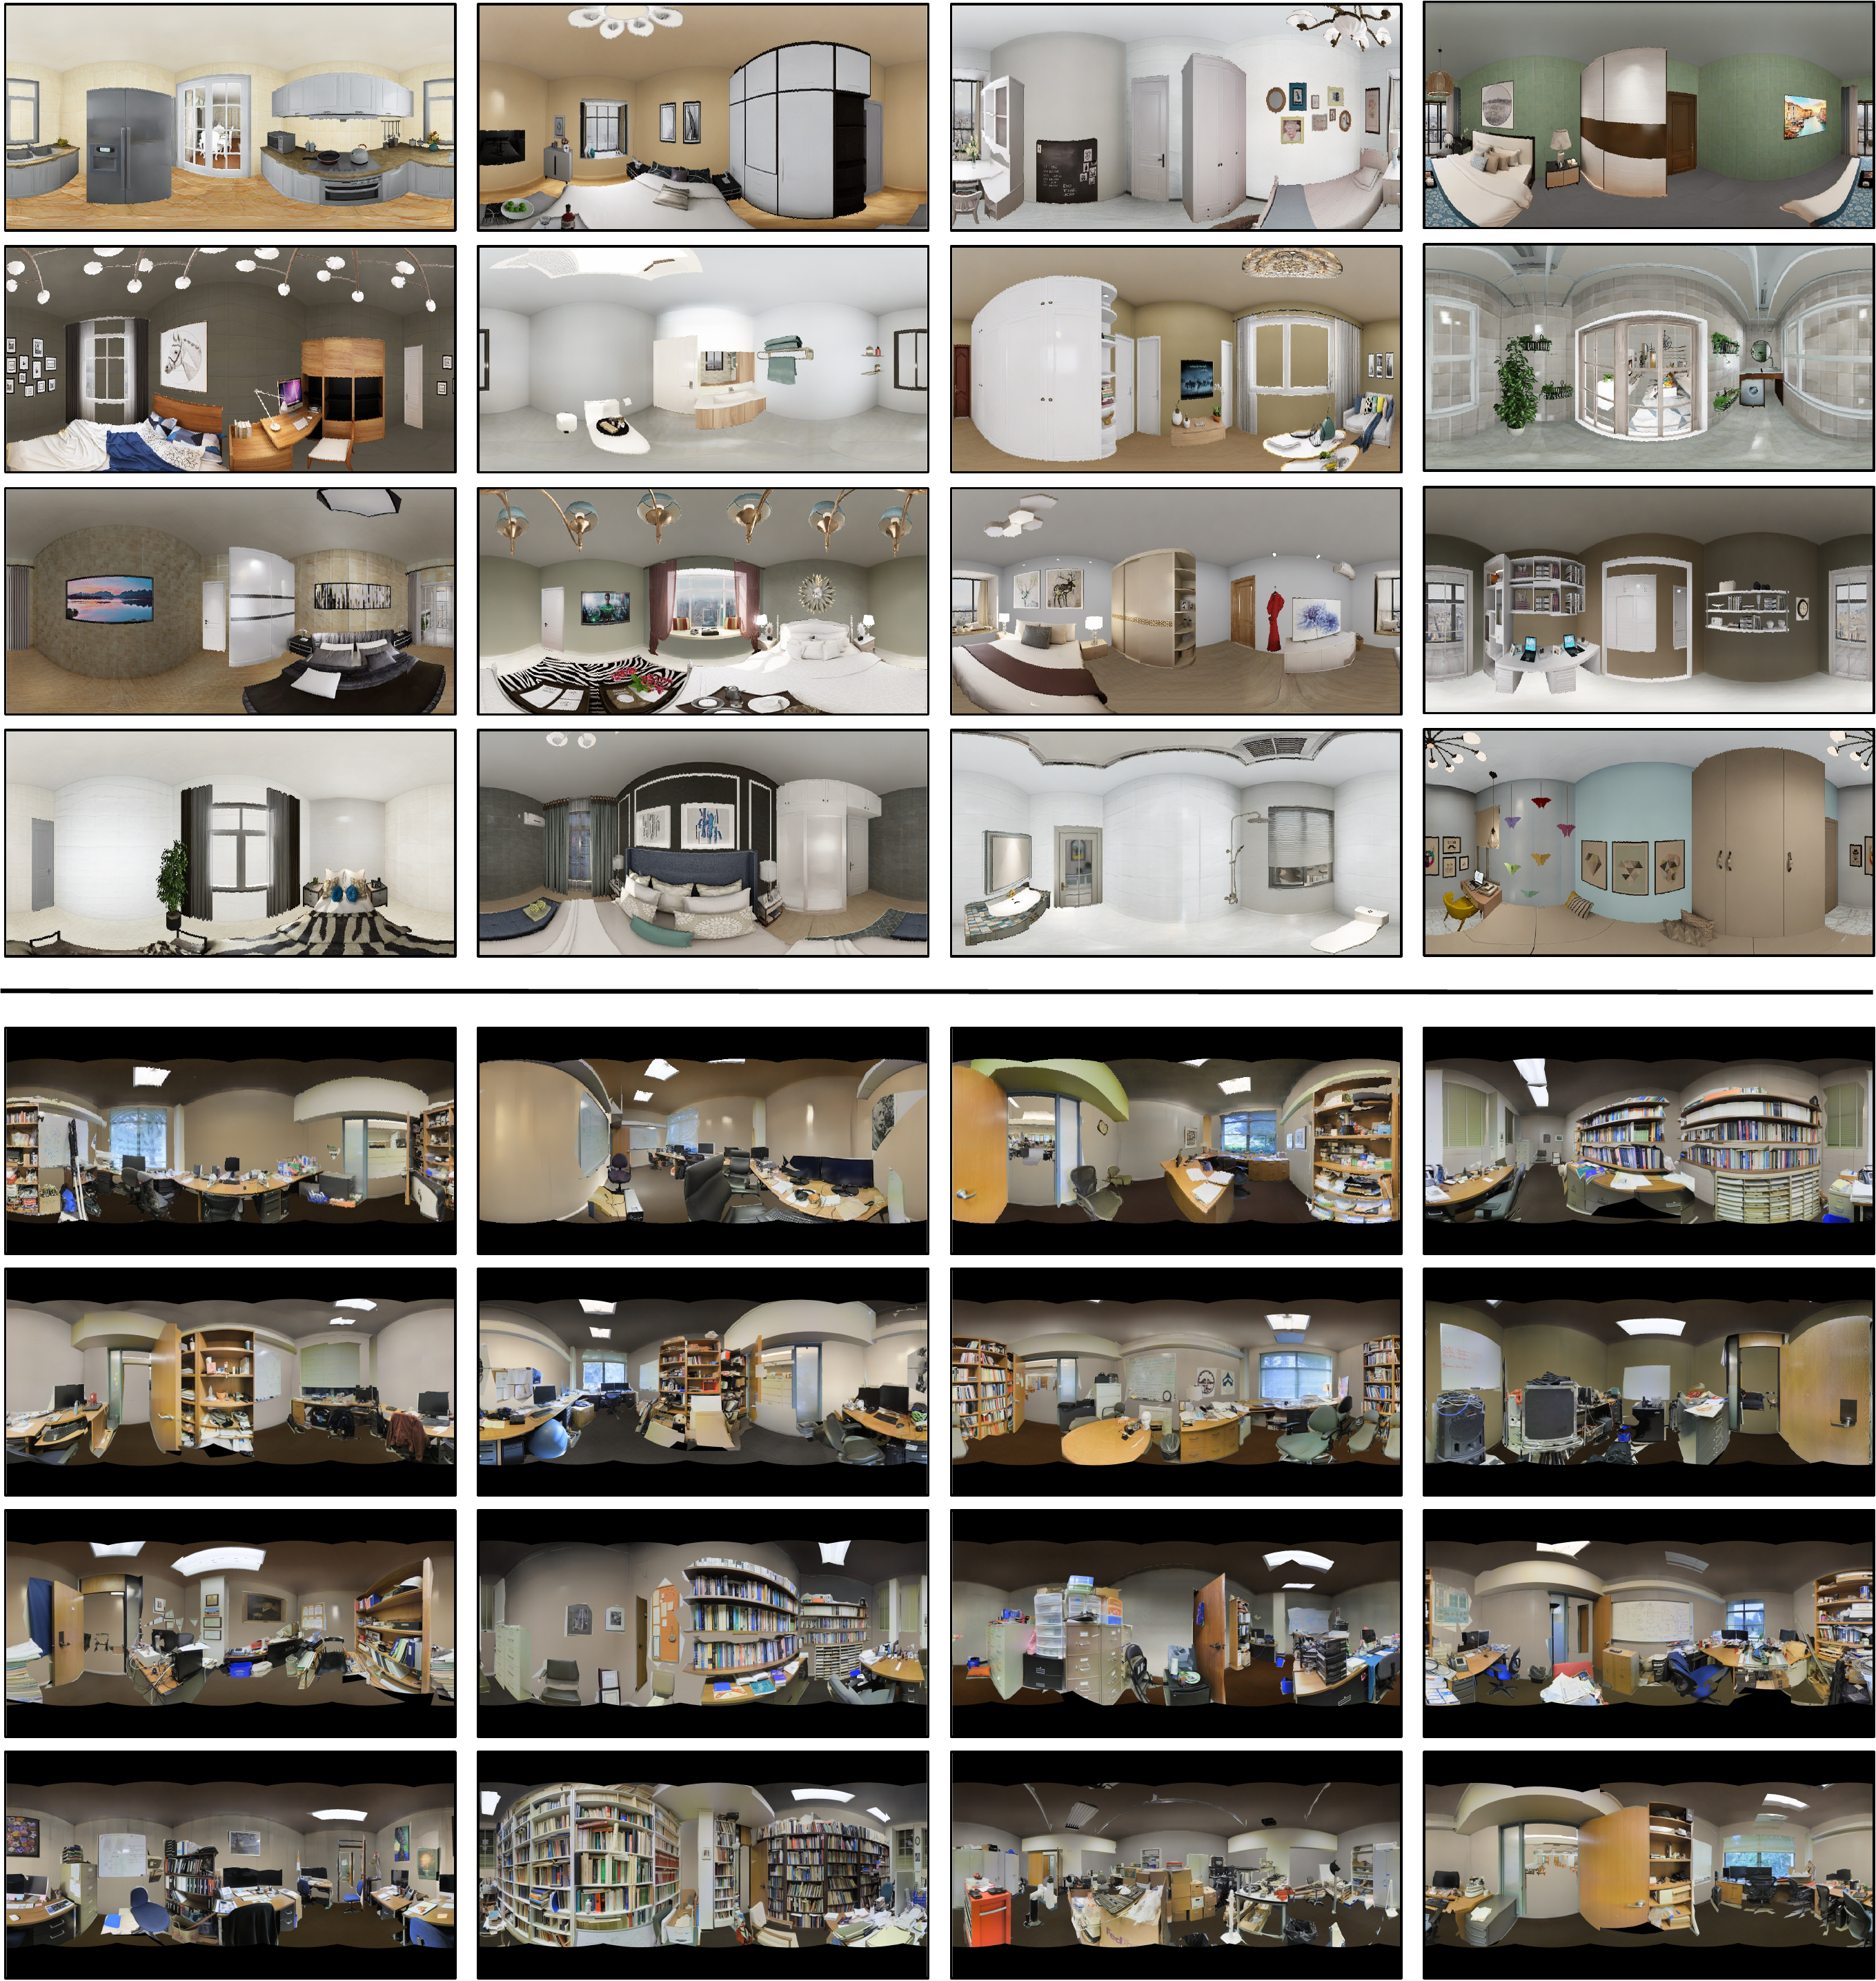}
  \caption{Qualitative results for Augmented images generated from Structured3D\cite{Structured3D} (upper part) and Stanford2D3D\cite{Stanford2D3D} (lower part) }
  \label{figure:qualitative result1}
\end{figure*}

\begin{figure*}
\includegraphics[scale=.255]{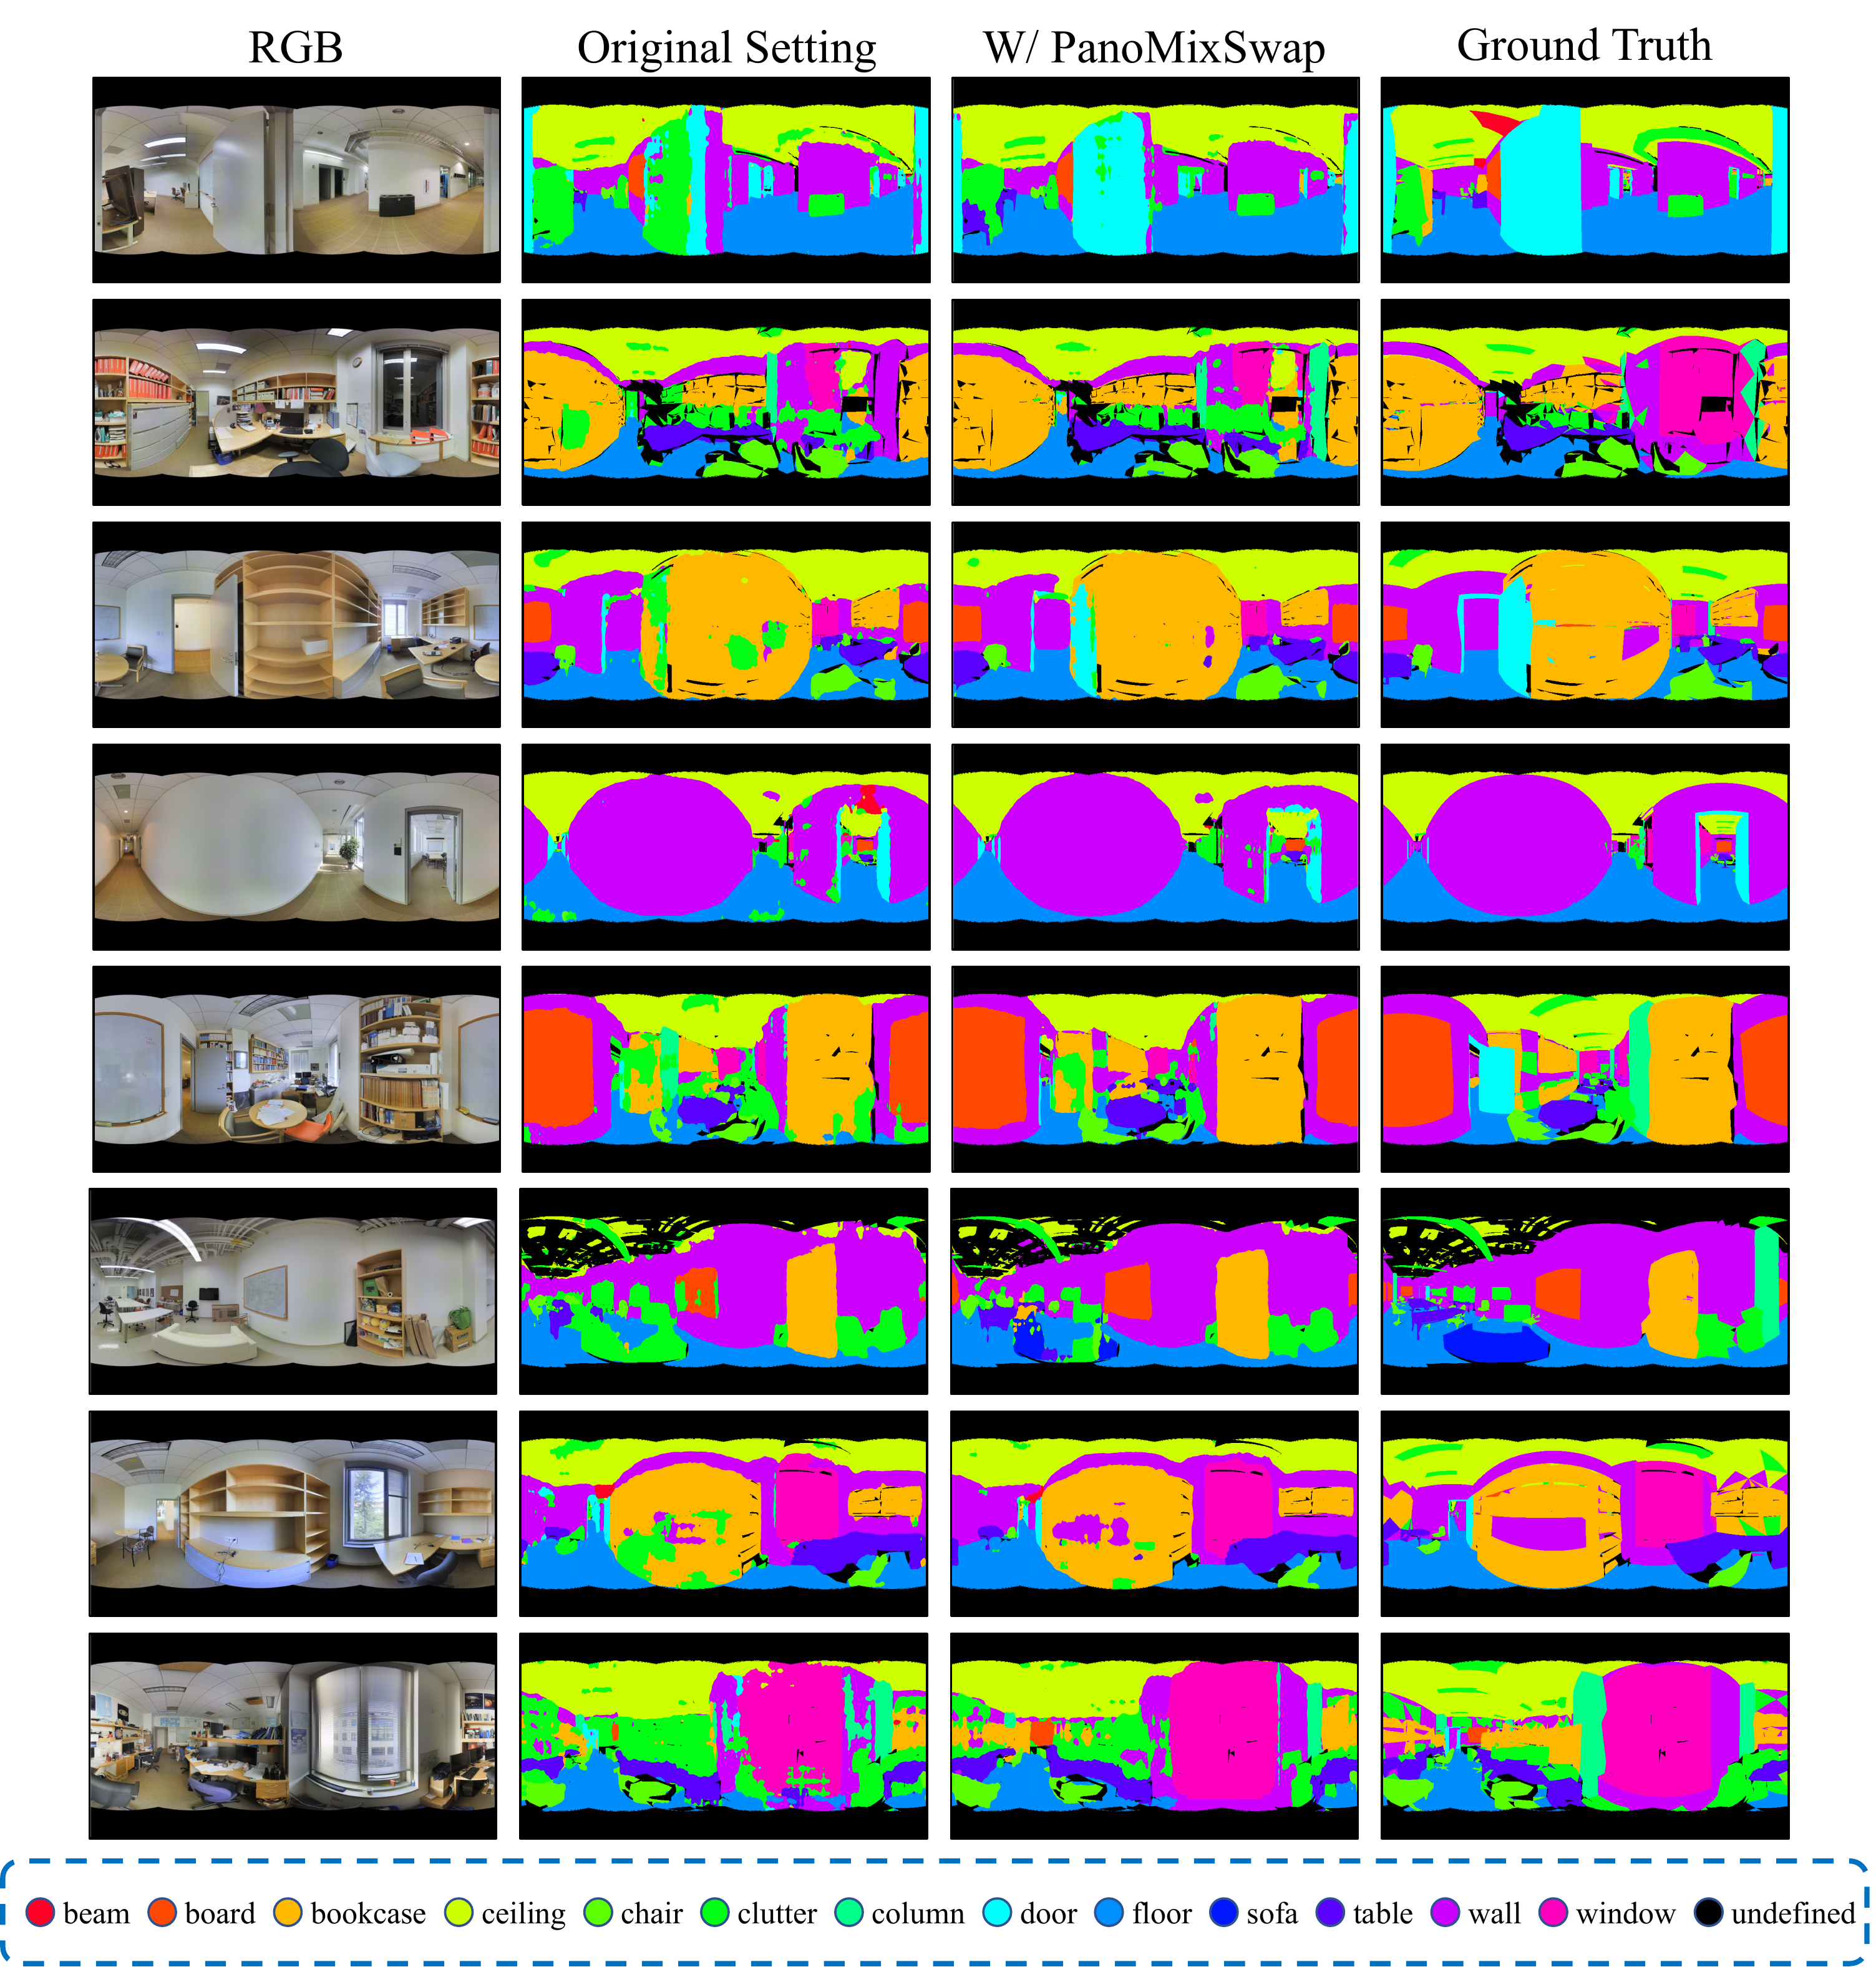}
  \caption{Qualitative results for semantic segmentation on Stanford2D3D\cite{Stanford2D3D}dataset.}
  \label{figure:sem_seg_s2d3d}
\end{figure*}

\begin{figure*}
\includegraphics[scale=.255]{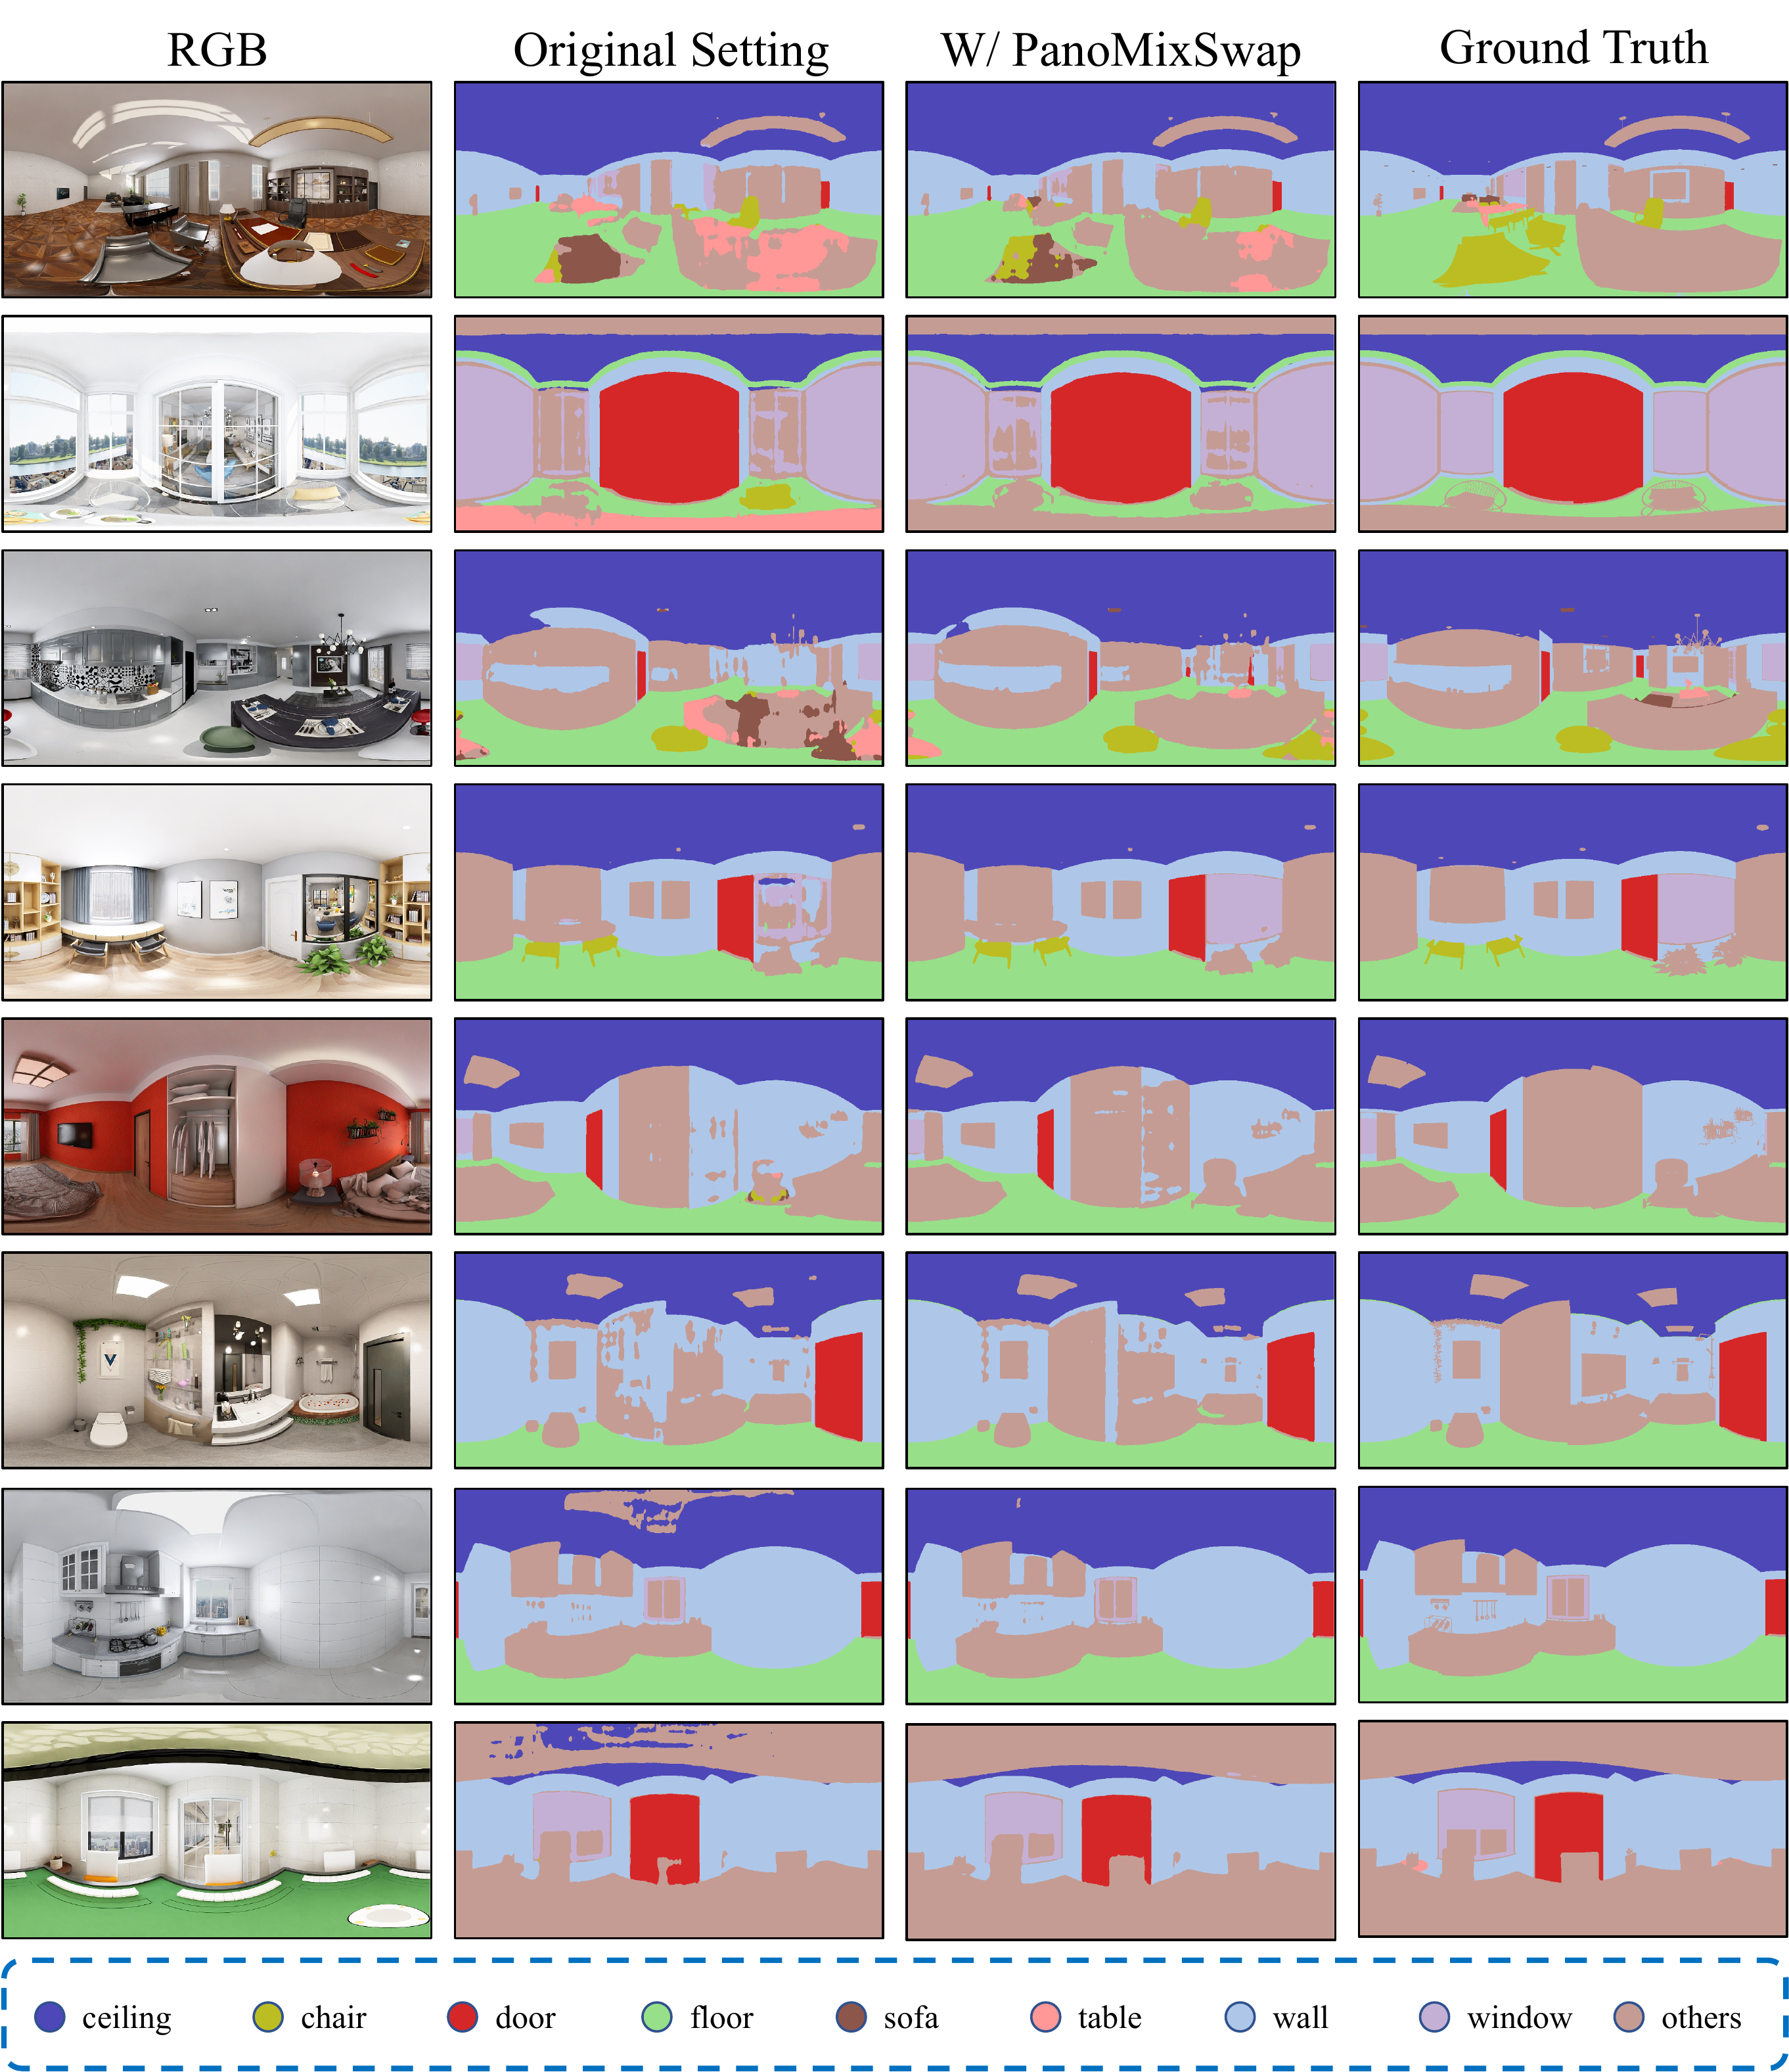}
  \caption{Qualitative results for semantic segmentation on Structured3D\cite{Structured3D}dataset.}
  \label{figure:sem_seg_Structured3D}
\end{figure*}

\begin{table}[htbp]
    \centering
    % \resizebox{0.99\linewidth}{!}{
    \begin{tabular}{cccc}
    \toprule
        PanoStretch & \modelname & mIoU(\%) & mACC(\%) \\ \midrule
        - & - & 52.00 & 65.00\\
        \checkmark & - & 53.63 & 65.06\\
        - & \checkmark & \textbf{56.02} & \textbf{67.43}\\
         \checkmark & \checkmark & 55.91 & 67.03\\
    \bottomrule
    \end{tabular}
    %}
    \caption{
    Quantitative comparison between two panoramic augmentation--- PanoStretch and \modelname on semantic segmentation task.}
    \label{tabel:Semantic Segmentation}
\end{table}
